# Supplementary material for: Controlling the coherence of a diamond spin qubit through strain engineering
Source: arXiv:1706.03881 source file (2018-01-31)
Supplement: Supplementary file 1 [file supp_final.pdf]

# Supplementary material for: Controlling the coherence of a diamond spin qubit through strain engineering

Young-Ik Sohn*[1], Srujan Meesala*[1], Benjamin Pingault*[2], Haig A. Atikian[1], Jeffrey Holzgrafe[1,2], Mustafa Gündoğan[2], Camille Stavrakas[2], Megan J. Stanley[2], Alp Sipahigil[3], Joonhee Choi[1,3], Mian Zhang[1], Jose L. Pacheco[4], John Abraham[4], Edward Bielejec[4], Mikhail D. Lukin[3], Mete Atatüre[2], and Marko Lončar[1]

[1]John A. Paulson School of Engineering and Applied Sciences, Harvard University, 29 Oxford Street, Cambridge, MA 02138, USA
[2]Cavendish Laboratory, University of Cambridge, J. J. Thomson Avenue, Cambridge CB3 0HE, UK
[3]Department of Physics, Harvard University, 17 Oxford Street, Cambridge, MA 02138, USA
[4]Sandia National Laboratories, Albuquerque, NM 87185, USA

## 1 Fabrication

The diamond NEMS (nano-electro-mechanical system) device used in this work was fabricated in three steps in the following order: (i) fabrication of bare diamond cantilevers, (ii) creation of silicon vacancy color centers, and (iii) deposition of electrodes. We use commercially available, ⟨100⟩-cut, ultra-high purity, single-crystal diamond (type IIa, nitrogen concentration less than 5 ppb) synthesized by chemical vapor deposition (CVD) [1].

Cantilevers are fabricated in two steps. First, diamond with patterned electron-beam resist is etched vertically with oxygen plasma [2]. These vertically-etched structures are then made free-standing by etching the sample at a tilted angle. Specifically, we employ an oxygen-plasma assisted ion-milling process in which the sample is mounted at an angle that is manually adjustable within a few degrees of precision. An illustration of this process, and the resulting suspended structure is schematically shown in Fig. S1(a).The etching occurs over a period of a few hours, during which the stage is rotated constantly. Further discussion

*These authors contributed equally

of these techniques can be found in [3, 4].

After cantilever fabrication, silicon ions ($Si^+$) are implanted at target spots on the cantilevers using a custom focused-ion-beam (FIB) system at Sandia National Labs. The spot size of the ion-beam on the sample is 40 nm, and is expected to determine the lateral precision of the implantation procedure. The beam energy is chosen to be 75 keV, which is predicted to yield a mean implantation depth of 50 nm with a straggle of 10 nm according to Stopping and Range of Ions in Matter simulations. Further details of the FIB implantation procedure can be found in [5, 6]. After FIB implantation, the sample is subjected to a tri-acid clean (1:1:1 sulfuric, perchloric, and nitric acids), and a three-step high-temperature high-vacuum annealing procedure [7, 8] in an alumina tube furnace. The annealing sequence followed comprises steps at 400°C (1.5°C per minute ramp, 8 hour dwell time), 800°C (0.5°C per minute ramp, 12 hour dwell time), and 1100°C (0.5°C per minute ramp, 2 hour dwell time). During the entire procedure, the pressure is maintained below $5 \times 10^{-7}$ torr. Annealing generates a small amount of graphite on the diamond surface, which is subsequently etched away by a tri-acid clean. Following this step, we perform a cleaning in piranha solution to ensure a high level of oxygen-termination at the diamond surface. With regards to conversion efficiency, we implant approximately 50 $Si^+$ ions per target spot on the sample, and typically generate 1-3 SiVs at each spot after annealing.

Subsequently, electrode patterns are made by a conventional bi-layer PMMA process followed by metal evaporation. Since the distance between the top surface of the cantilever and the bottom substrate is approximately $4\,\mu$m, bi-layer PMMA is spun multiple times until the cantilevers are buried completely. Patterns are written by electron-beam lithography, and metals are evaporated to define the electrodes. Detailed fabrication steps are schematically shown in Fig. S1(b). Here, the triangle represents the cantilever, and the pedestal to the right of the triangle is the location of the bonding pad for electrical contact. The bi-layer PMMA process is repeated twice - first, to define the bonding pad, and second, to define the electrode pattern near the cantilever. This is because, we use a 200 nm thick gold layer for the bonding pad, but only a 10 nm thick tantalum (Ta) layer for the cantilever electrodes. Fig. S1(c) shows the scheme to connect electrodes on top of the cantilevers to the bonding pad on the diamond pedestal. Electrodes on the substrate below the cantilevers are connected to a second bonding pad (now shown in the figure) that is directly on the surface of the diamond.

We now discuss the choice of 10 nm tantalum film for our cantilever electrodes. For five different metals we have tested as a cantilever electrode material (aluminium, chromium, copper, titanium and tantalum), our device always shows a continuous, non-zero leakage-current upon applying voltage. While the exact reasons for this leakage-current on our sample, in particular, are unknown, there have been numerous studies on the surface conductivity of diamond under various conditions [9]. For aluminium, chromium, copper and titanium, this leakage current destroys the electrode when a high voltage (in the few hundred volts range) is applied. The destruction of electrodes appeared to be the result of melting or bursting of the thin metal film, likely caused by Joule heating [10]. Tantalum is one of the metals with the highest melting and evaporation points among those available for e-beam evaporation. We find that devices with tantalum electrodes are robust enough to operate at very high

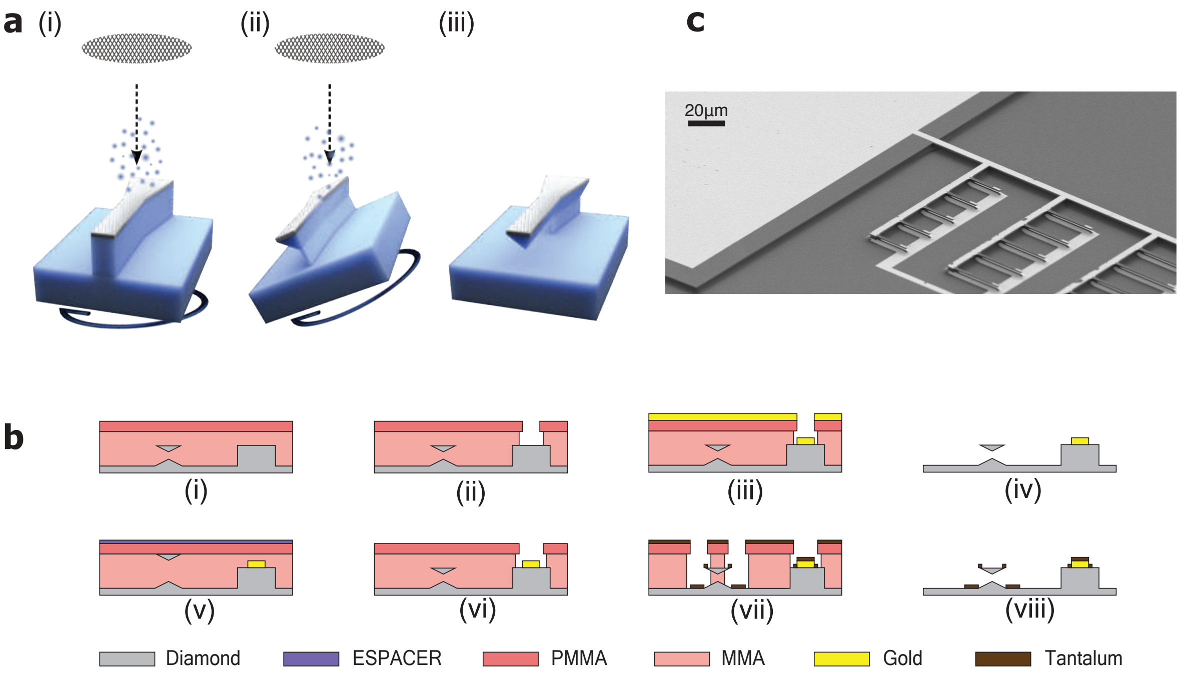


Figure S1: (a) Schematic of oxygen-plasma assisted ion-milling process for angled-etching of diamond cantilevers. The ion beam is directed at the diamond sample, with a vertically-etched device pattern. The tilted stage is continuously rotated during the etching process. After the cantilevers are freely standing, the etch-mask is stripped. (b) Fabrication process for the placement of electrodes. First, the coarsely aligned bonding pad is defined with a bi-layer PMMA process followed by gold evaporation. Then the same process is repeated to define tantalum electrodes near cantilevers, but with better alignment precision. Conductive layer (ESPACER 300Z) on top of the cantilever is helpful for precise alignment. (c) SEM image of the complete chip showing connection between the bonding pad and electrodes on top of the cantilevers.

applied voltage ($\sim$600 V across an electrode gap of approximately 4 $\mu$m, which corresponds to an electric-field of 1.5 MV/cm). The thickness of tantalum is kept below 10 nm in order to avoid thin film-induced stress in the cantilever, which leads to pre-strained SiV centers.

# 2 Device design

An important figure of merit for our NEMS device is the maximum achievable strain at the location of SiV. In this section, we discuss two key design aspects that need to be considered towards this goal: (i) 'pull-in instability', and (ii) practical limits for high voltage operation.

Pull-in instability is a well-known phenomenon for an electrostatic actuator made with a parallel plate capacitor as shown in Fig. S2(a). In these devices, voltage is applied to induce an electrostatic force between two plates, where either one or both of them are free to move. Upon applying a voltage, the capacitor deforms until it reaches equilibrium, when there is a

balance between the electrostatic force, and the restoring force exerted by the elasticity of the material. The net force acting on the free top plate in Fig. S2(a) can be modeled as

$$F(x,V) = -\frac{\partial U(x,V)}{\partial x} = \frac{1}{2}\varepsilon A \frac{V^2}{(d-x)^2} - kx \tag{1}$$

where $x$ is the displacement of the plate, $U(x,V)$ is the potential energy and $\varepsilon$ is the permittivity of the material between the two plates. $A$ is the area of the capacitor, $V$ is the voltage applied, $d$ is the distance between the two plates at 0 V, and $k$ is the spring constant, respectively. By integrating equation (1), we can calculate $U(x,V)$ at various voltages as shown in Fig. S2(b). The local minimum in the potential represents a condition of stable equilibrium. As the voltage is increased, the local minimum shifts towards the bottom plate, indicating that the top plate gets displaced downwards, thereby reducing the capacitor gap. When the voltage changes from $3V_0$ to $4V_0$ in the Fig. S2(b), the stable local minimum disappears. This occurs, when the top plate is displaced by about one-third of the initial gap between the two plates, i.e. when $x = d/3$. At this point, the system reaches a condition in which the top plate snaps down to the bottom plate. Our device is a slight variation of this conceptual model, and hence, the maximum deflection of our cantilever will be limited by pull-in instability (but not at exactly $x = d/3$).

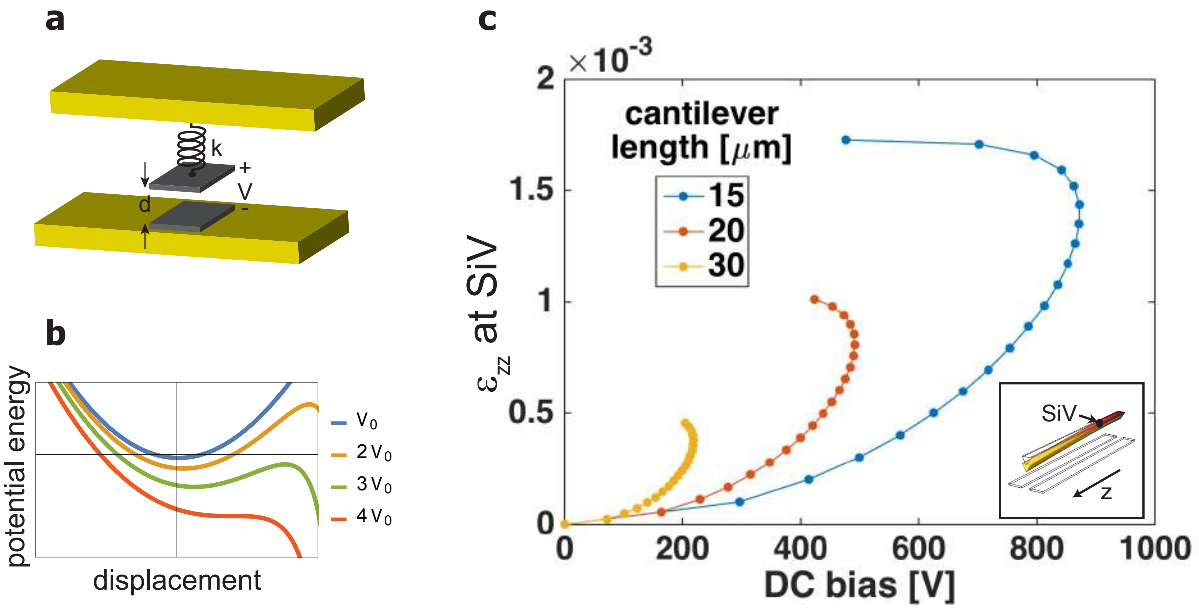


Figure S2: (a) Illustration of a parallel plate capacitor with one freely movable plate (top), and one fixed plate (bottom). The top electrode can be actuated by applying a voltage. (b) Potential energy of the system in (a) with the different voltages. The stable minimum in the potential disappears, when the system reaches the condition of pull-in instability at a voltage of $4V_o$. (c) FEM simulation of the strain-component along the long-axis of the cantilever (most dominant strain-tensor component) near the clamp of the cantilever (inset). Turnaround points in the graph represent pull-in instabilities.

A 3D finite element method (FEM) calculation can be used to simulate pull-in instability accurately for complex structures [11]. Typically, a simulation can be run by setting a particular voltage on the electrode, and solving for the resultant deformation of the structure, thereby arriving at the strain profile inside the cantilever. One can also run the inverse of this procedure. By setting a target displacement of the cantilever tip, the voltage required to achieve this displacement can be calculated. Such an inverse calculation can help arrive at the condition for pull-in instability. Fig. S2(c) shows the results of a simulation run so as to solve this inverse problem. Strain at the SiV location is plotted as a function of the voltage for different cantilever lengths. Turnaround points represent the pull-in instability condition at which both the displacement of the cantilever-tip and the applied voltage reach the maximum value possible before the cantilever snaps down. Fig. S2(c) provides two important conclusions: First, for a given voltage, longer cantilevers provide larger strain for a given voltage, because they have a smaller spring constant. Second, the maximum attainable strain is higher for shorter cantilevers, because they reach the pull-in instability condition at a higher voltage. Therefore, shorter devices are preferred to generate high strain, when arbitrarily high voltage can be applied.

In practice, however, there are mechanisms that limit the maximum possible voltage e.g. Townsend breakdown, field emission and surface current [12, 13, 14], all of which can be significant depending on experimental conditions. With the fabrication method described in Section 1, our devices could be operated safely up to voltage as high as 600 V under high vacuum ($\sim 10^{-7}$ torr) at cryogenic temperature (4 K). Given that the minimum electrode gap is 4 $\mu$m, this condition corresponds to an electric field of approximately 1.5 MV/cm. Experiments described in Section 7 are carried out in a helium closed-cycle cryostat with the sample surrounded by helium exchange gas at a pressure of 1 mbar. Under these conditions, we observed safe operation up to 500 V. The maximum voltage in this setup is thought to be limited by dielectric breakdown of helium gas.

Considering all the design limitations discussed above, we chose cantilevers of width 1.2-1.3 $\mu$m and length 25-30 $\mu$m for the experiments in this work.

# 3 Strain-dependent photoluminescence measurements

The sample is cooled down to a nominal temperature of 6 K inside a Janis ST-500 continuous helium-flow cryostat. The cryostat is mounted under a home-built scanning confocal microscope with a 0.9 NA 100×, 1 mm working distance objective (Olympus MPLFLN 100X) housed inside the cryostat. SiV centers are identified via non-resonant excitation with a 703 nm laser diode (Thorlabs LP705-SF15), and collection of zero-phonon-line (ZPL) fluorescence in a narrow bandwidth of 10 nm around 737 nm. For resonant photoluminescence excitation (PLE) of ZPL transitions, we use a tunable continuous-wave Ti-sapphire laser (M-Squared Solstis), and collect the resulting fluorescence in the phonon-sideband (above 750 nm). Mode-hop-free tuning of the laser is achieved over the scan range of interest by using feedback from a wavemeter (High Finesse WS7). A CW 532 nm laser is periodically pulsed using an acousto-optic modulator (Crystal Technology 3080) to maintain the negative charge

state of SiV(-) centers [5]. Collected fluorescence (gated off during green excitation) is sent to an avalanche-photodiode to measure the photon-count rate. DC voltage for cantilever-deflection is supplied from a Stanford Research Systems PS300 high-voltage source. As an added precautionary measure, the weak leakage-current in the circuit (typically below 100 nA) discussed in Section 2 is monitored via a Keithley 2400 source-meter. Strain-response measurements involve taking resonant excitation spectra as the voltage applied to the device is steadily increased. Such a sequence of spectra is shown in Fig. S3, and is used to derive Fig. 2a in the main text. Strain corresponding to the applied voltage is estimated through finite element method (FEM) simulations [15].

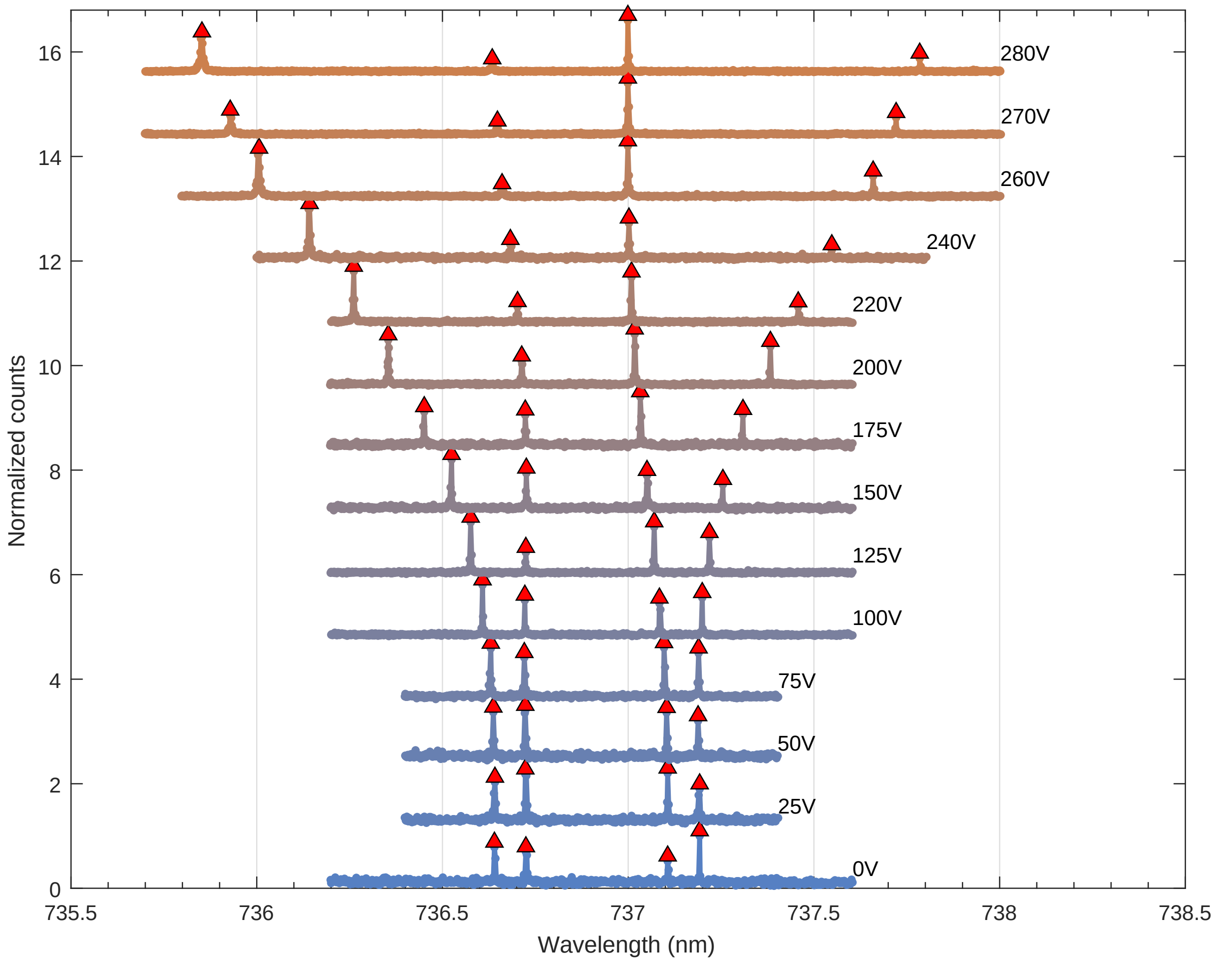


Figure S3: PLE spectra of an SiV center with increasing voltage applied to the device

# 4 High-strain PLE spectra

In our devices, we can generate uniaxial strain as high as $\sim 10^{-3}$ at a voltage of 600 V. Example spectra showing strain-tuning into this regime are shown in Fig. S4. At high strain, as $\Delta_{gs} \gg k_B T \sim 80\,\text{GHz}$ at $T = 4\,\text{K}$, population in the upper branch $|2\rangle$ of the ground-state man-

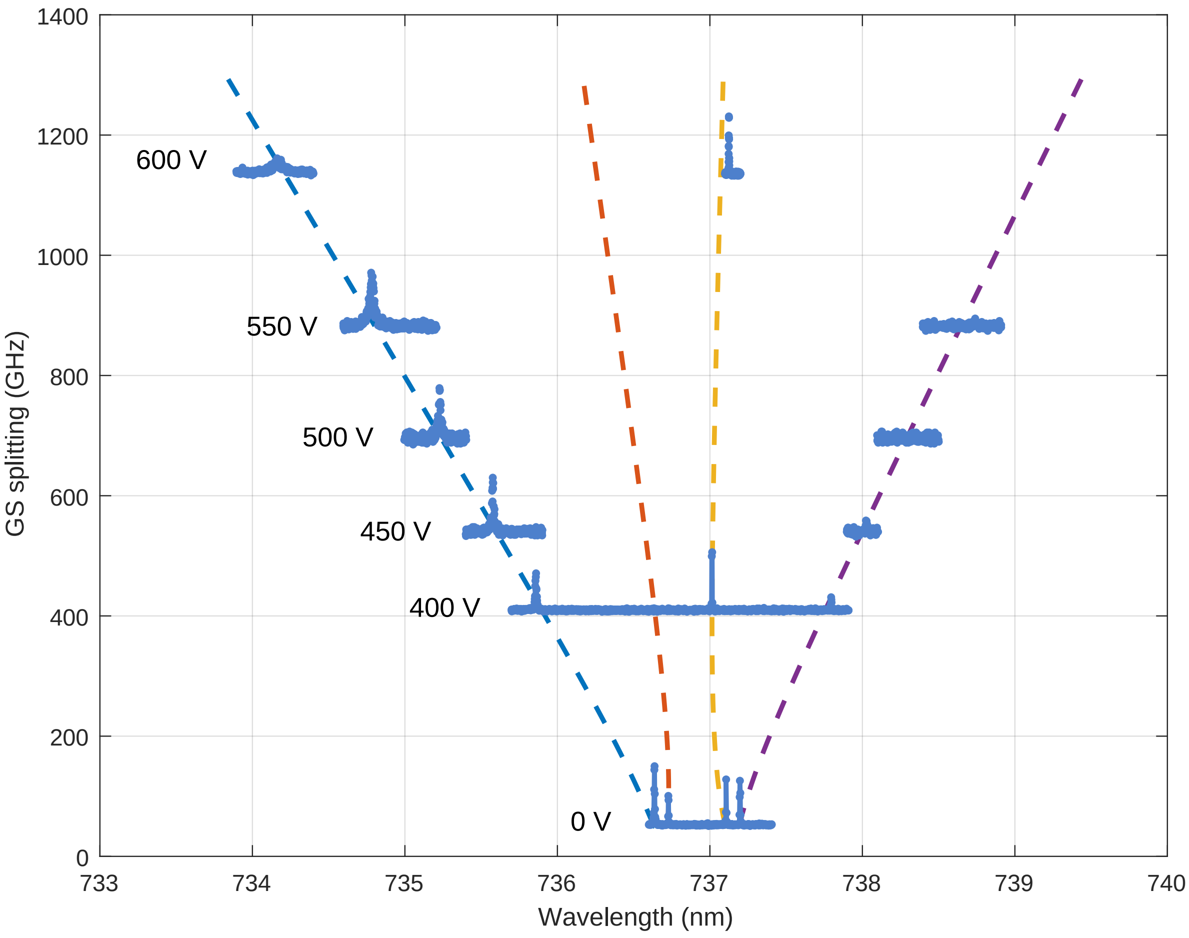


Figure S4: Tuning of PLE spectrum of a transverse SiV subject to high strain. Voltage applied to the device is indicated next to each spectrum. $y$-axis shows ground-state splitting $\Delta_{\rm gs}$ corresponding to the spectrum estimated using the procedure detailed in the text. Dashed lines correspond to modeled strain-response of the four optical transitions.

ifold decreases exponentially, while the population in the lower branch $|1\rangle$ correspondingly increases to near-unity. As a result, with increasing strain, the B and D transitions become weaker in intensity, and eventually vanish. Simultaneously, the linewidth of the A transition increases owing to increasingly rapid phonon-mediated relaxation in the excited state from $|4\rangle$ to $|3\rangle$. This is captured by the model for single-phonon emission and absorption discussed in Section 6. On the other hand, as the C transition connects the lower orbitals in ground and excited states ($|1\rangle$ and $|3\rangle$), its linewidth is not affected as strongly by phonon-mediated processes, and is measured to be relatively unchanged with strain (See Section 9). The C transition also becomes brighter at high-strain due to near-unity population in the lower ground state branch $|1\rangle$.

While the high-strain spectra only reveal A and C transitions, the difference in their frequencies gives us the excited-state splitting $\Delta_{\rm es}$ exactly. Since the same strain-components are responsible for increasing $\Delta_{\rm gs}$ and $\Delta_{\rm es}$, we can use the strain-susceptibilities in [16, 15] to

estimate $\Delta_{gs}$. Using this procedure, for the highest strain condition in Fig. S4, we infer $\Delta_{gs}$ = 1.2 THz. A more precise experimental technique to measure the GS- and ES-splittings at high strain is described in Section 7.3.

# 5 Orbital thermalization measurements

We use time resolved pump-probe fluorescence to characterize the phonon processes in the GS. In this method, two consecutive laser pulses resonant with the D transition are used to, first initialise GS orbital population in the lower branch $|1\rangle$, and after a set delay $\tau$, read-out population in the upper branch $|2\rangle$. A schematic of the pulse sequence, and an example of a resulting fluorescence time-trace are shown in Fig. S5. By repeating this sequence for steadily increasing pump-probe delay $\tau$, we measure the rate at which the GS population relaxes towards thermal equilibrium due to resonant phonons.

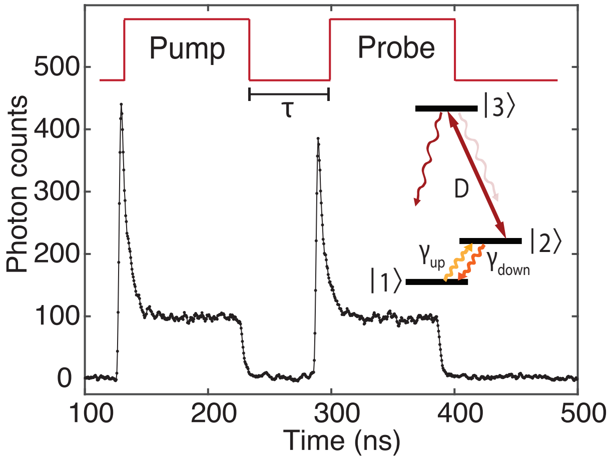


Figure S5: Time-resolved fluorescence signal in pump-probe measurement for a delay $\tau = 50$ ns between the two laser pulses. The laser is resonant with the D transition, and optically pumps the GS population into the lower orbital branch $|1\rangle$ over a timescale of few ns. After time $\tau$, the fluorescence signal from the probe pulse has a leading edge determined by the population in the upper orbital branch $|2\rangle$. The decay rates between levels $|1\rangle$ and $|2\rangle$ - $\gamma_{up}$ due to phonon-absorption, and $\gamma_{down}$ due to phonon-emission - are also shown.

## 5.1 Experimental setup

The pump-probe pulse sequence described above is implemented by pulsing our resonant-excitation laser with a Mach-Zehnder intensity electro-optic modulator (EO Space AZ-AV5-5-PFA-PFA-737) driven by a digital-delay generator with rise- and fall-times of 2 ns (SRS DG645). Over the course of the measurements, the operation point of the intensity electro-optic modulator (EOM) is stabilized against long-term drifts with continuous feedback on the DC-bias voltage. The feedback loop is implemented with a lock-in amplifier (SRS SR830) generating a low-frequency (1 KHz) modulation of the DC-bias voltage. Photon-count pulses

from the single-photon-detector are time-tagged on a PicoHarp 300 module triggered by the delay-generator. The laser frequency itself is stabilized by continuous feedback with a wavemeter (High Finesse WS7).

## 5.2 Extraction of thermalization rate

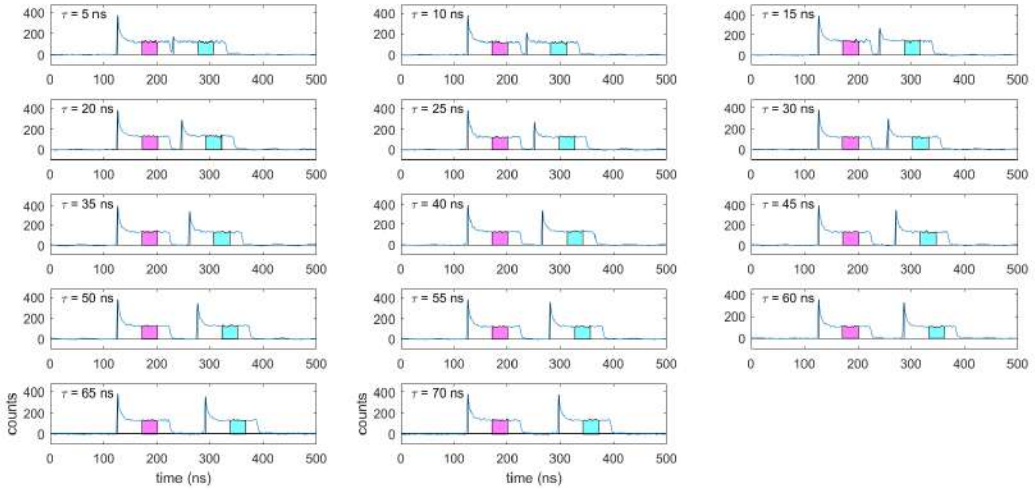


Figure S6: Fluorescence time-traces for various pump-probe delays between $\tau$=5 ns to 70 ns taken at GS-splitting $\Delta_{\mathrm{gs}}$=46 GHz. $x$-axis is time in ns, and $y$-axis is photon counts integrated over multiple iterations of the pulse sequence.

Example data from implementing the pulse sequence in Fig. S5 for various pump-probe delays is shown in Fig. S6. This data can be interpreted and processed to yield a GS-population thermalization curve as follows. As shown in Fig. S7a, the leading edge of the first fluorescence signal corresponds to thermal population $p_{2,th}$ in the GS level $|2\rangle$. Upon switching on the pump pulse, this decays to a residual value $p_{2,opt}$ determined by the competition between the optical pumping rate (above saturation, this is simply the decay rate $\gamma_e$ from the excited state $|3\rangle$) and the rates $\gamma_{\mathrm{up}}, \gamma_{\mathrm{down}}$. After time delay $\tau$, the leading edge of the probe fluorescence signal corresponds to partially recovered population $p_2(\tau)$ due to thermalization. We can describe the population recovery in level $|2\rangle$ as

$$(p_2(\tau) - p_{2,th}) = (p_2(\tau) - p_{2,opt}) \exp\left[-\left(\gamma_{\mathrm{up}} + \gamma_{\mathrm{down}}\right) t\right] \tag{2}$$

In particular, we calculate the normalized change in photon-counts, $(p_2(\tau) - p_{2,th}) / (p_2(\tau) - p_{2,opt})$ from each measurement in Fig. S6, and carry out an exponential fit in Fig. S7b to extract $(\gamma_{\mathrm{up}} + \gamma_{\mathrm{down}})$. Repeating this experiment for various values of GS-splitting $\Delta_{\mathrm{gs}}$, we arrive at Fig. 2c in the main text.

From the optical-pumping fluorescence signal, we can define a pumping efficiency $\left(1 - \frac{p_{2,opt}}{p_{2,th}}\right)$. This describes the ability of the pump pulse to initialize GS population in level $|1\rangle$ by

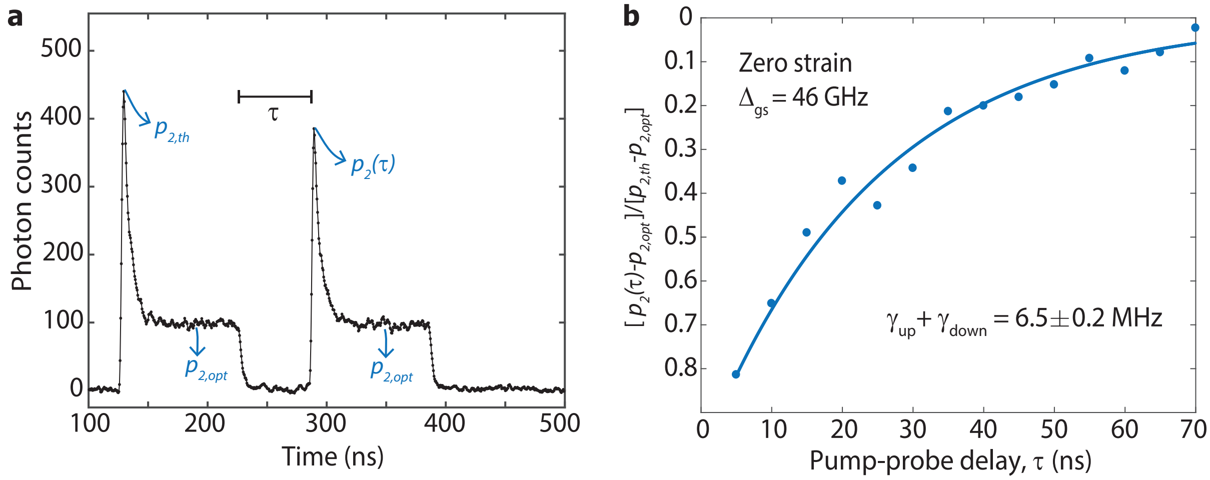


Figure S7: (a) Fluorescence time-trace for $\tau$=50 ns from Fig. S6 showing relevant quantities related to the population in level $|2\rangle$. (b) Thermalization curve constructed by extracting the normalized change in photon-counts for various pump-probe delays $\tau$. Solid line is an exponential fit.

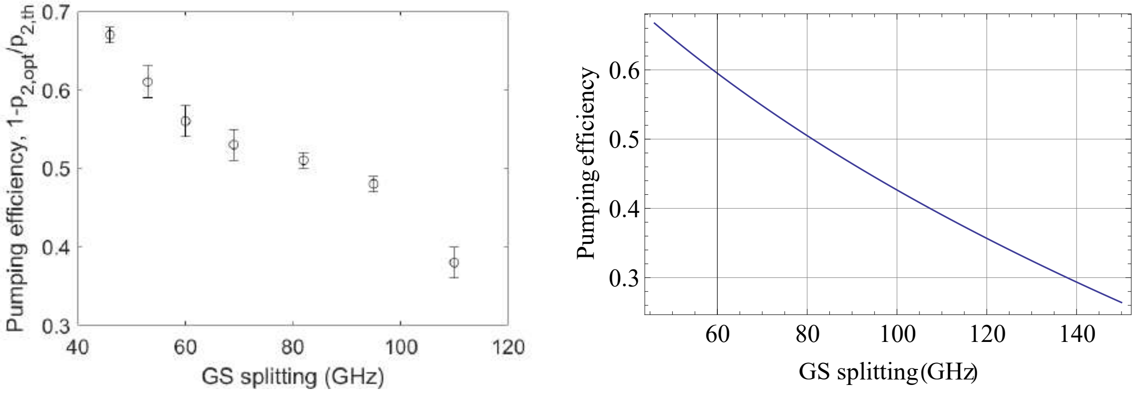


Figure S8: (a) Experimentally measured optical-pumping efficiency (see text for definition) versus GS-splitting $\Delta_{gs}$. (b) Theoretically estimated optical-pumping efficiency using a three-level rate equations model. We assume optical pumping above saturation, GS thermalization rates, $\gamma_{up}$ and $\gamma_{down}$ to follow the model in Section 6, excited state decay rate $\gamma_e = 90$ MHz, branching ratio into $|1\rangle = 0.5$.

acting against the thermalization process. As the GS-splitting $\Delta_{gs}$ is increased, we find that the pumping-efficiency decreases in Fig. S8. This can be attributed to the downward thermalization rate $\gamma_{down}$ rapidly increasing with $\Delta_{gs}$ as will be discussed in Section 6. At large $\Delta_{gs}$, the optical pumping rate, $R_{opt}$, which is $\sim \gamma_e$, the excited state decay rate cannot substantially outweigh $\gamma_{down}$. As a result, the GS population cannot be optically pumped into level $|1\rangle$ better than is dictated by thermal equilibrium. This makes it impractical to measure the thermalization rate beyond a certain $\Delta_{gs}$ using the pump-probe technique. In our experiments, we measure up to $\Delta_{gs} = 110$ GHz.

# 6 Orbital thermalization model

## 6.1 Theory

Due to the nature of the strain interaction, phonons that are resonant with the ground state splitting $\Delta_{\text{gs}}$ can directly drive the orbital transition [17]. The transition rates driven by the continuum of lattice phonon modes can be calculated using Fermi's golden rule [18] to get:

$$\gamma_{\text{up}}(\Delta_{\text{gs}}) = 2\pi\chi\rho\Delta_{\text{gs}}^3 n_{th}(\Delta_{\text{gs}}) \tag{3}$$

$$\gamma_{\text{down}}(\Delta_{\text{gs}}) = 2\pi\chi\rho\Delta_{\text{gs}}^3 (n_{th}(\Delta_{\text{gs}}) + 1) \tag{4}$$

where $\rho$ is a constant proportional to average speed of sound in bulk, $n_{th}$ is the number of thermal phonons per mode and $\chi$ is the interaction frequency for a single phonon. In these expressions, the first term in the product, $2\pi\chi\rho\Delta_{\text{gs}}^3$ corresponds to the mean-squared single-phonon coupling rate multiplied with the DOS at the GS splitting $\Delta_{\text{gs}}$, while the second term corresponds to the thermal occupation of each mode. Fig. S9 shows plots of the calculated dependence of upward and downward rates on $\Delta_{\text{gs}}$ at temperature $T = 4\,\text{K}$. We observe that the upward rate shows a non-monotonic behavior, approaching its maximum value around $h\Delta_{\text{gs}} \sim k_B T$. The increasing DOS term dominates in the regime $h\Delta_{\text{gs}} < k_B T$, and causes $\gamma_{\text{up}}$ to increase. However, when $h\Delta_{\text{gs}} \gg k_B T$, the thermal occupation of the modes behaves as $n_{th}(\Delta_{\text{gs}}) = \exp\left(-\frac{h\Delta_{\text{gs}}}{k_B T}\right)$. This exponential roll-off dominates the polynomially increasing DOS, and causes $\gamma_{\text{up}}$ to decrease at higher strain. In contrast, the downward rate monotonically increases with the GS-splitting, because it is dominated by the spontaneous emission rate, which simply scales as the DOS.

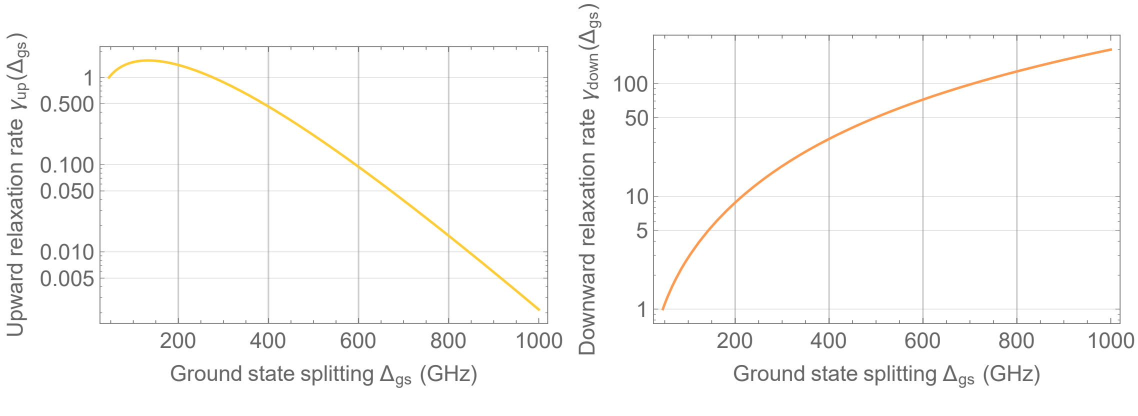


Figure S9: Variation of the upward (phonon-absorption) and downward (phonon-emission) relaxation rates with GS-splitting $\Delta_{\text{gs}}$ at temperature $T$=4 K. The $y$-axis is normalized to the zero-strain rates $\gamma_{\text{up}}(46\text{GHz})$ and $\gamma_{\text{down}}(46\text{GHz})$ in each plot respectively.

## 6.2 Fitting

With the pump-probe technique used in our experiments, we measure the sum of the upward and downward rates, which should have the dependence

$$\gamma_{\mathrm{up}}(\Delta_{\mathrm{gs}}) + \gamma_{\mathrm{down}}(\Delta_{\mathrm{gs}}) = A\Delta_{\mathrm{gs}}^3(2n_{th}(\Delta_{\mathrm{gs}}) + 1) = A\Delta_{\mathrm{gs}}^3 \coth\left(\frac{h\Delta_{\mathrm{gs}}}{k_B T}\right) \tag{5}$$

where $A$ is a constant. Our cantilever has lateral dimensions of order $1\,\mu$m. This is about an order of magnitude larger than half the acoustic wavelength for $\Delta_{\mathrm{gs}} = 50\,\mathrm{GHz}$ in diamond, which is $\sim$120 nm. Thus, the cantilever itself is a bulk-like structure for the SiV. However, as can be observed in the left panel of Fig. S10 our experimental data shows very poor agreement with the theoretically predicted behavior in equation (5).

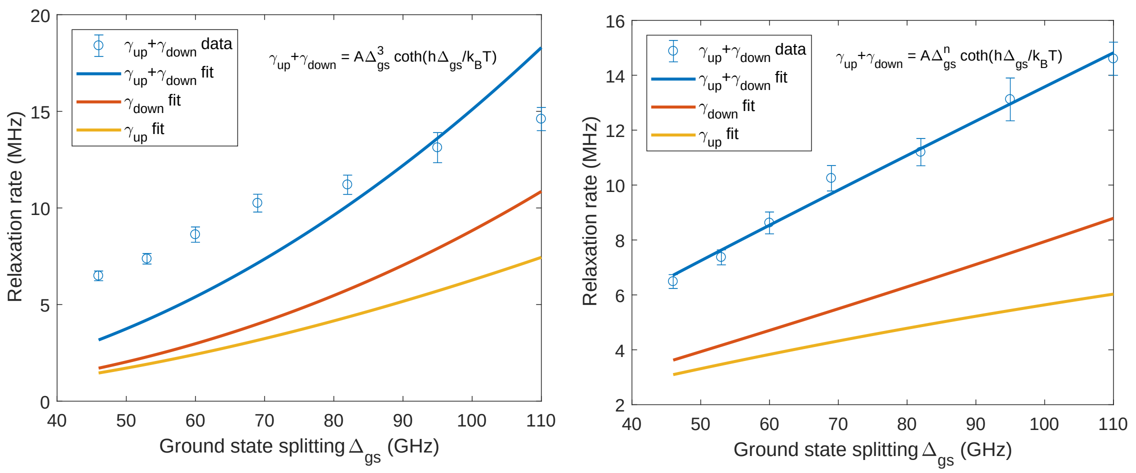


Figure S10: Fits to experimental measurements of net orbital thermalization rate $\gamma_{\mathrm{up}} + \gamma_{\mathrm{down}}$ (solid blue line) assuming coupling to only bulk acoustic modes (left plot), and unknown DOS behavior (right plot) with varying $n$. Fit expressions are indicated in top left corner of each plot. Corresponding individual rates $\gamma_{\mathrm{up}}$ and $\gamma_{\mathrm{down}}$ are extracted and plotted after fitting in each case (solid yellow and orange lines). The fit to variable DOS (right plot) yields $n = 1.9 \pm 0.3$.

Instead, when we allow the exponent of the DOS term to be a variable $n$, we obtain a better fit yielding $n = 1.9 \pm 0.3$. We can arrive at a possible explanation for this discrepancy, if we note that the SiV is situated at a nominal depth of 50 nm, which is sub-wavelength for phonons in the frequency range of $\Delta_{\mathrm{gs}}$ probed in our experiment. As a result, we can expect appreciable coupling to surface acoustic modes, which are not accounted for in the above derivation. Since the DOS of surface modes scales as $\Delta_{\mathrm{gs}}^2$, it appears that the thermalization rate in our experiment is almost entirely determined by surface modes.

# 7 SiV spin measurement techniques

## 7.1 Experimental setup

The sample is cooled down to a temperature of 3.8 K inside a closed cycle liquid helium cryostat (Attodry 1000). It is placed in a dip stick, in which helium gas (pressure $\sim 1$ mbar) acts as an exchange gas. Two superconducting coils surrounding the sample chamber can be used to apply a magnetic field along two orthogonal axes, up to 8 T vertically and up to 2 T horizontally. DC voltage for cantilever-deflection is supplied by a high-voltage source (Stanford Research Systems PS310/1250V-25W). As an added precautionary measure described in Section 3, the weak leakage-current in the circuit (typically below 100 nA) is monitored via a Keithley 2400 source-meter. The optical part of the setup consists of a home-built confocal microscope mounted on top of the cryostat, and a microscope objective (NA = 0.82) inside the sample chamber. The sample is mounted on piezoelectric stages (Attocube ANPx101 and ANPz101) allowing to position the sample with respect to the objective. Non-resonant excitation of SiVs is performed using a diode laser at 660 nm (Laser Quantum Ventus), while resonant excitation is achieved with a tunable diode laser around 737 nm (Toptica DLpro). The frequency of the latter is stabilised through continuous feedback from a wavemeter (High Finesse WSU).

## 7.2 Coherent-population-trapping

For coherent population trapping (CPT), sidebands are generated on the resonant excitation laser using an EOM (Photline NIR-MX800) connected to a tunable microwave source (Rhode&Schwarz SMF 100A). Fluorescence from the emitters is collected through the microscope objective. A 750 nm long-pass filter in the confocal microscope allows collection of the phonon-sideband emission from $SiV^-$ centres, filtering out the laser excitation. This emission is then sent to an avalanche photodiode (APD) (Excellitas). This measurement is repeated for different values of ground state splitting, the results of which constitute Figs. 4b and 4c of the main text.

## 7.3 Calibration of ground and excited state splittings with applied voltage at high strain

The ground state splitting can be measured directly by considering the energy difference between the transitions labelled C and D in Fig. 2(a) of the main text. Due to the presence of other $SiV^-$ centres generated at the same spot due to the FIB implantation procedure, measuring this energy difference between C and D transitions through non-resonant PL spectra is impractical. At the same time, simultaneous detection of C and D transitions through resonant excitation is not possible at high strain, since the Boltzmann population in level $|2\rangle$ becomes negligible as discussed in Section 4. To overcome this limitation, we resonantly excite transition A of the SiV center being studied, and record the spectrum of transitions C and D on a spectrometer after having filtered out the resonant laser with a monochromator. The spectra are then fitted with two Lorentzian functions to extract the value of the ground state splitting, as shown in Fig. S11. Likewise, the excited state

splitting (also shown in the figure) can be derived as the difference between the frequencies of transitions A and C in this measurement.

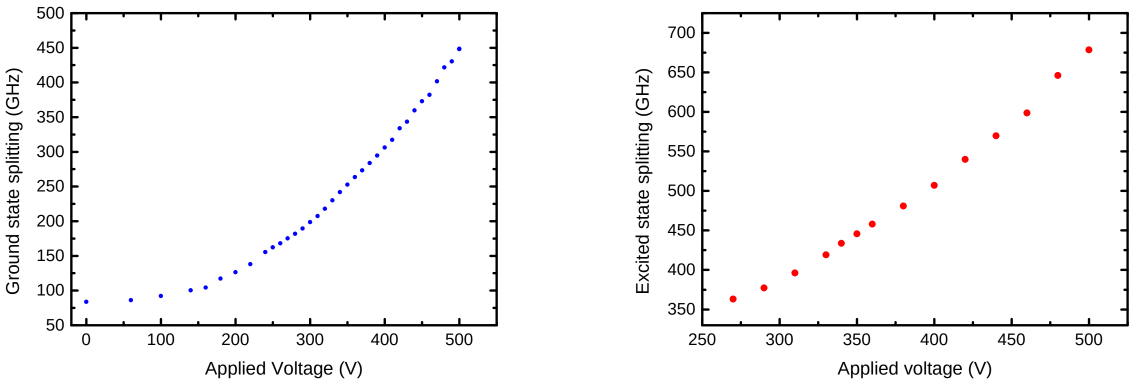


Figure S11: SiV ground state splitting (left), and excited state splitting (right) measured as a function of voltage applied to the cantilever. Error bars are smaller than the dots and correspond to the standard deviation on the frequency difference between C and D transitions estimated from Lorentzian fits.

# 8 Investigation of double-dip CPT signal

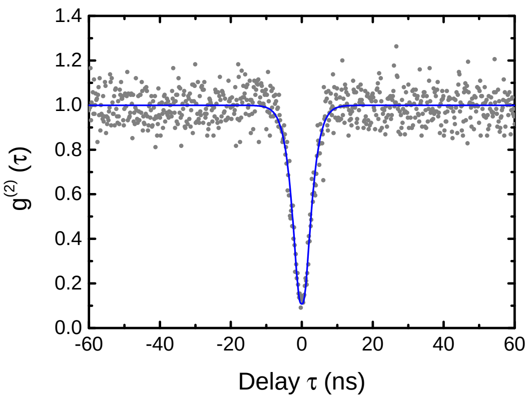


Figure S12: Second-order correlation measurement of the $SiV^-$ centre investigated. The measured data points are plotted as grey dots. A fit based on a three-level model and accounting for timing jitter is plotted as a blue curve.

We first rule out the hypothesis that the two dips in our CPT measurements originate from two different SiV centres. The dips are very similar in width and depth, and their frequency-separation remains constant ($4.0 \pm 0.1$ MHz) over a wide range of applied strain (see Fig. 4b of main text). In the event that this is caused by two SiV centers, they are required to have the same fluorescence intensity, and experience exactly the same strain conditions at

any applied voltage, which is very unlikely. In order to categorically establish that we are investigating a single SiV centre, we perform a Hanbury-Brown-Twiss (HBT) experiment on the phonon-sideband fluorescence upon resonant excitation of transition C, and measure the second order correlation function $g^{(2)}$ as shown in Fig. S12. The $g^{(2)}$ function is fitted using a three-level model described in [19] convolved with the Gaussian response of the avalanche photodiodes used, which have a timing jitter of 350 ps. At zero time delay, a clear anti-bunching reaching $g^{(2)}(\tau = 0) = 0.12$ indicates that the measured photons originate from a single emitter.

To gain more insight into the origin of the two CPT dips, we perform CPT at varying orientation of the applied magnetic field, while keeping its magnitude (0.2 T) constant. We work in the high-strain regime at a ground state splitting of 467 GHz. In our results, shown in Fig. S13, we observe that the separation between the two CPT dips displays a periodic variation as the magnetic field is rotated.

Given the similarity of the two dips, a very plausible explanation for the double-dip structure is the presence of a proximal spin in the environment of the SiV centre being studied. Physically, varying the direction of the applied B-field leads to a variation in the quantization axis of the SiV electron-spin (or semi-classically, the orientation of the electron magnetic moment). Likewise, the quantization axis of the proximal spin has its own variation with the B-field orientation. For instance, if this proximal spin is a nuclear spin, to first order, its orientation simply follows that of the applied B-field. As a result, the dipole-dipole interaction energy of the SiV electron-spin with the neighboring spin varies with B-field orientation, leading to the periodic behavior observed experimentally in Fig. S13. Below, we describe a semi-classical approach to model the CPT dip separation as a dipole-dipole interaction.

The Hamiltonian for two dipoles with magnetic moments $\boldsymbol{\mu_1}$ and $\boldsymbol{\mu_2}$ is given by

$$\mathbb{H}^{\text{d-d}} = -\frac{\mu_0}{4\pi\left|\mathbf{r}\right|^3}\left(3\left(\boldsymbol{\mu_1}\cdot\hat{\mathbf{r}}\right)\left(\boldsymbol{\mu_2}\cdot\hat{\mathbf{r}}\right) - \boldsymbol{\mu_1}\cdot\boldsymbol{\mu_2}\right) \tag{6}$$

where $\mu_0$ is the vacuum-permeability, $\mathbf{r}$ is the vector from one dipole to the other, and $\hat{\mathbf{r}}$ is given by $\mathbf{r}/\left|\mathbf{r}\right|$. If the two dipoles are spins described by spin angular momentum $\mathbf{S}_1$ and $\mathbf{S}_2$, we can write the interaction Hamiltonian in terms of the spin-operators.

$$\mathbb{H}^{\text{d-d}} = -\frac{\mu_0\gamma_1\gamma_2}{4\pi\left|\mathbf{r}\right|^3}\left(3\left(\mathbf{S}_1\cdot\hat{\mathbf{r}}\right)\left(\mathbf{S}_2\cdot\hat{\mathbf{r}}\right) - \mathbf{S_1}\cdot\mathbf{S_2}\right) \tag{7}$$

where $\gamma_i$ is the gyromagnetic ratio of spin $i$. Semi-classically, we can treat spin angular momentum as a vector quantity $\mathbf{S} = \frac{\hbar}{2}\left(\langle\sigma_x\rangle, \langle\sigma_y\rangle, \langle\sigma_z\rangle\right)$, where $\sigma_x, \sigma_y, \sigma_z$ are Pauli spin-matrices. This vector describes the mean-orientation of the electron magnetic moment. To calculate the SiV electron-spin orientation under our experimental conditions, the full ground-state Hamiltonian including spin-orbit coupling, external strain, and magnetic field must be diagonalized. The effect of the external magnetic field is described by the Zeeman Hamiltonian below written in the basis $\{|e_X,\uparrow\rangle, |e_X,\downarrow\rangle, |e_Y,\uparrow\rangle, |e_Y,\downarrow\rangle\}$ [20],

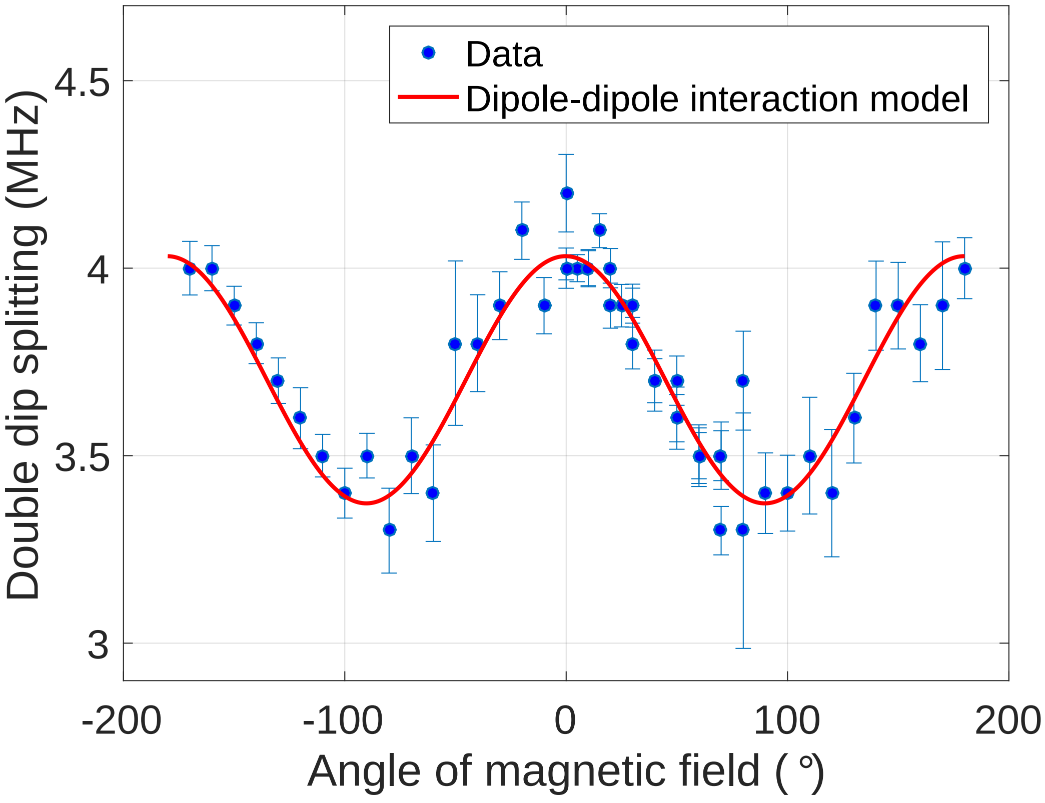


Figure S13: Dependence of CPT dip separation on magnetic field orientation. The angle plotted on the $x$-axis is measured with respect to the vertical direction on the sample. $0°$ corresponds to the [001] axis of diamond, while $90°$ corresponds to the [110] axis of diamond, along which the cantilever long-axis is aligned. The SiV investigated is a transverse SiV, so its internal $Z$-axis is either $[1\bar{1}1]$ or $[\bar{1}11]$. Error bars correspond to the standard deviation on the CPT dip frequencies estimated from Lorentzian fits.

$$\mathbb{H}^{\text{Zeeman}} = q\gamma_L \hat{L}_z B_z + \gamma_S \hat{\mathbf{S}} \cdot \mathbf{B} = q\gamma_L \begin{bmatrix} 0 & 0 & iB_z & 0 \\ 0 & 0 & 0 & iB_z \\ -iB_z & 0 & 0 & 0 \\ 0 & -iB_z & 0 & 0 \end{bmatrix} + \gamma_S \begin{bmatrix} B_z & B_x - iB_y & 0 & 0 \\ B_x + iB_y & -B_z & 0 & 0 \\ 0 & 0 & B_z & B_x - iB_y \\ 0 & 0 & B_x + iB_y & -B_z \end{bmatrix} \quad (8)$$

where the first and second terms are from the orbital angular momentum, and the spin angular momentum, respectively. $\hat{L}_z$ and $\hat{S}$ are $L_z$ and $\mathbf{S}$ normalized by $\hbar$, respectively. The gyromagnetic ratios for each term are given by $\gamma_L = \mu_B/\hbar$, $\gamma_S = 2\mu_B/\hbar$, where $\mu_B$ is the

Bohr magneton. $q$ is a quenching factor that is commonly observed in solid-state emitters [17].

The total Hamiltonian $\mathbb{H}^{\text{total}}$ is obtained by adding the spin-orbit Hamiltonian $\mathbb{H}^{\text{SO}}$ and strain Hamiltonian $\mathbb{H}^{\text{strain}}$.

$$\mathbb{H}^{\text{total}} = \mathbb{H}^{\text{SO}} + \mathbb{H}^{\text{strain}} + \mathbb{H}^{\text{Zeeman}} \tag{9}$$

$$\mathbb{H}^{\text{SO}} + \mathbb{H}^{\text{strain}} = \begin{bmatrix} \alpha - \beta & 0 & \gamma - i\lambda_{SO}/2 & 0 \\ 0 & \alpha - \beta & 0 & \gamma + i\lambda_{SO}/2 \\ \gamma + i\lambda_{SO}/2 & 0 & \alpha + \beta & 0 \\ 0 & \gamma - i\lambda_{SO}/2 & 0 & \alpha + \beta \end{bmatrix} \tag{10}$$

$\lambda_{SO}$, the spin-orbit coupling is 46 GHz for the ground state of the SiV. $\alpha$, $\beta$, and $\gamma$ are strain tensor components obeying the symmetries of the SiV center as defined in [15, 20]. We diagonalize the total Hamiltonian, $\mathbb{H}^{\text{total}}$, and calculate expectation values of the Pauli matrices for the lowest two eigenstates, which comprise the SiV spin-qubit under investigation. This gives us the mean orientation of the SiV electron-spin, say $\mathbf{S}_1$ for given experimental conditions. To calculate the mean orientation of the proximal spin $\mathbf{S}_2$, we assume it to be either a nuclear spin such as $^{13}$C, or an electron spin such as another SiV-center. In the case of a nuclear spin, $\mathbf{S}_2$ is simply given by the direction of the external magnetic field. Once the quantization axes of the two spins are known, we can fit our data to the calculated value of $\mathbb{H}^{\text{d-d}}$ from Eq. 7 by using the distance between the spins $\mathbf{r}$ as a fit parameter. The result of such a fitting procedure is shown in Fig. S13. In the case of a nuclear spin, the distance between the two spins $|\mathbf{r}|$ is estimated to be on the order of 1 Å. If the other spin is an electron spin from another SiV centre, it is possible to obtain similar results as in Fig. S13. However, in this case, the distance between the spins is on the order of tens of nanometres.

# 9 Spectral diffusion of C transition

The C transition of the SiV centre used in our CPT measurements does not experience extra spectral diffusion at high strain (high voltage). In theory, there are two potential causes of spectral diffusion that might appear at high strain. (i) A gradient of strain could perturb the inversion symmetry of the SiV-center, and induce a nonzero permanent dipole moment for the electronic levels. (ii) A large DC-electric field at the SiV location arising from the applied voltage could induce a linear Stark shift response to fluctuating electric-fields in the environment of the SiV, thereby increasing spectral diffusion. In our experiments, the amount of spectral diffusion on the timescale of minutes (roughly $\pm$20 MHz) does not appear to increase from the zero-voltage to the high-voltage condition (Fig. S14). This is further confirmed by our measurements of the C transition linewidth at various high strain conditions. (Fig. S15). We do observe a systematic drift in the transition frequency on the timescale of hours, but this slow drift can be easily corrected for by adjusting the resonant laser excitation frequency (or alternatively by performing feedback on the DC voltage applied to our device).

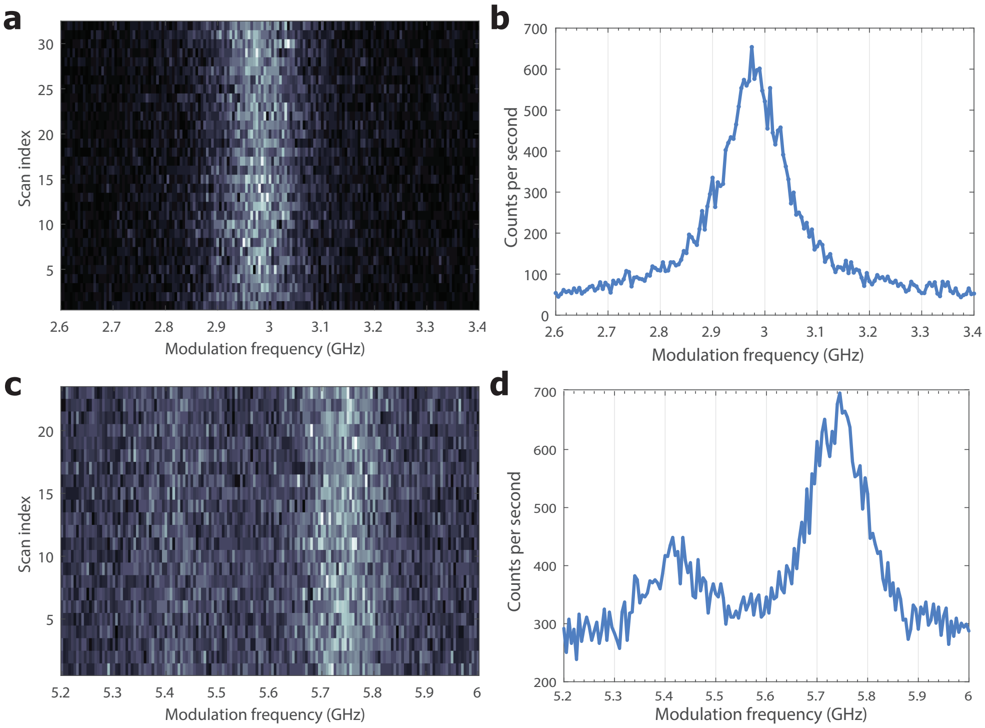


Figure S14: (a) Continuous monitoring of the resonant excitation spectrum of the C transition at 0 V (ground state splitting of 88 GHz) and 0 T. Each horizontal line corresponds to a single acquisition of the spectrum over a duration of 0.6 s with 5 MHz spectral resolution. (b) Average of the 32 scans in part (a) corresponding to a total acquisition time of 20 s (c) Continuous monitoring of the resonant excitation spectrum of two of the four Zeeman-split C transitions at 400 V (ground state splitting of 303 GHz) and a B-field of 0.2 T. Each horizontal line corresponds to a single acquisition of the spectrum over a duration of 0.6 s with 5 MHz spectral resolution. (d) Average of the 23 scans in part (c) corresponding to a total acquisition time of 14 s.

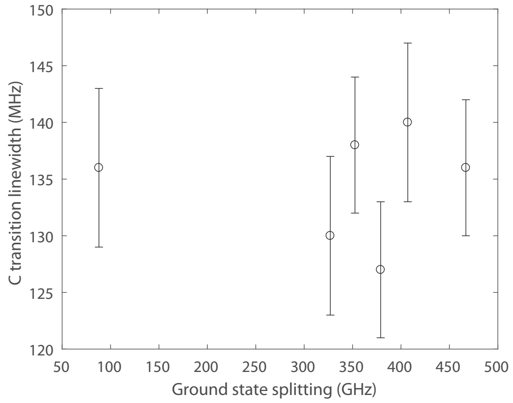


Figure S15: Linewidth of the C transition measured at various strain conditions over a timescale of few minutes. Error bars are obtained from Lorentzian fits to the spectra.

# References


[1] element six ™ (2017). URL http://www.e6.com.

[2] Hausmann, B. J. M. *et al.* Fabrication of diamond nanowires for quantum information processing applications. *Diamond & Related Materials* **19**, 621–629 (2010).

[3] Atikian, H. A. *et al.* Wafer-scale fabrication of freestanding nanostructures via reactive ion beam undercut etching (2017).

[4] Burek, M. J. *et al.* Free-Standing Mechanical and Photonic Nanostructures in Single-Crystal Diamond. *Nano Letters* **12**, 6084–6089 (2012).

[5] Sipahigil, A. *et al.* Supplementary materials - an integrated diamond nanophotonics platform for quantum-optical networks. *Science* **354**, 847–850 (2016).

[6] Schröder, T. *et al.* Scalable focused ion beam creation of nearly lifetime-limited single quantum emitters in diamond nanostructures. *arXiv:1610.09492 [quant-ph]* (2016).

[7] Chu, Y. *et al.* Coherent optical transitions in implanted nitrogen vacancy centers. *Nano Letters* **14**, 1982–1986 (2014).

[8] Evans, R. E., Sipahigil, A., Sukachev, D. D., Zibrov, A. S. & Lukin, M. D. Narrow-linewidth homogeneous optical emitters in diamond nanostructures via silicon ion implantation. *Phys. Rev. Applied* **5**, 044010 (2016).

[9] Maier, F., Riedel, M., Mantel, B., Ristein, J. & Ley, L. Origin of surface conductivity in diamond. *Phys. Rev. Lett.* **85**, 3472–3475 (2000).

[10] Chen, K. C.-Y. *et al.* Conductor fusing and gapping for bond wires. *Progress In Electromagnetics Research M* **31**, 199–214 (2013).

[11] Comsol multiphysics® v. 5.2. URL www.comsol.com.

[12] Zhan, S., Azarian, M. H. & Pecht, M. G. Surface insulation resistance of conformally coated printed circuit boards processed with no-clean flux. *IEEE transactions on electronics packaging manufacturing* **29**, 217–223 (2006).

[13] Townsend, J. S. (Oxford University Press, 1915).

[14] Strong, F. W., Skinner, J. L., Dentinger, P. M. & Tien, N. C. Electrical breakdown across micron scale gaps in mems structures. In *MOEMS-MEMS 2006 Micro and Nanofabrication*, 611103–611103 (International Society for Optics and Photonics, 2006).

[15] Meesala, S. *et al.* Strain engineering of the silicon vacancy center in diamond. *arXiV pre-print* arXiV 1801.09833 (2018).

[16] Sternschulte, H., Thonke, K., Sauer, R., Münzinger, P. C. & Michler, P. 1.681-eV luminescence center in chemical-vapor-deposited homoepitaxial diamond films. *Phys. Rev. B* **50**, 14554–14560 (1994).

[17] Hepp, C. *Electronic Structure of the Silicon Vacancy Color Center in Diamond*. Ph.D. thesis (2014).

[18] Jahnke, K. D. *et al.* Electron–phonon processes of the silicon-vacancy centre in diamond. *New Journal of Physics* **17**, 1–11 (2015).

[19] Neu, E. *et al.* Single photon emission from silicon-vacancy colour centres in chemical vapour deposition nano-diamonds on iridium. *New Journal of Physics* **13**, 025012 (2011).

[20] Hepp, C. Electronic structure of the silicon vacancy color center in diamond. *PhD dissertation* (2014).
